# Supplementary material for: ARRAKIS: Atlas of Resonance Rings As Known In the S4G
Source: arXiv:1312.0866 source file (2015-08-28)
Supplement: Supplementary file 1 [file appendixb.tex]

\clearpage
\onecolumn
\section{Double NGC and IC identifications}

\begin{table}[h]
 \caption{List of ARRAKIS galaxies with a double NGC/IC identification}
 \begin{tabular}{l l | l l}
 \hline\hline
ID used in the S$^4$G & Alternative ID & ID used in the S$^4$G & Alternative ID\\
\hline
IC~1826&IC~1830&            NGC~4336&IC~3254\\
IC~3102&NGC~4223&           NGC~4342&IC~3256\\
NGC~723&NGC~724&          NGC~4351&NGC~4354\\
NGC~755&NGC~763&          NGC~4355&NGC~4418\\
NGC~1291&NGC~1269&          NGC~4405&IC~788\\
NGC~1367&NGC~1371&          NGC~4413&NGC~4407\\
NGC~1415&IC~1983&           NGC~4461&NGC~4443\\
NGC~1425&IC~1988&           NGC~4492&IC~3438\\
NGC~1436&NGC~1437&          NGC~4591&NGC~4577\\
NGC~1448&NGC~1457&          NGC~4618&IC~3667\\
NGC~1452&NGC~1455&          NGC~4625&IC~3675\\
NGC~2604&NGC~2604A&         NGC~4722&IC~3833\\
NGC~2974&NGC~2652&          NGC~4845&NGC~4910\\
NGC~3301&NGC~3760&          NGC~4961&NGC~4960\\
NGC~3321&NGC~3322&          NGC~5334&IC~4338\\
NGC~3389&NGC~3373&          NGC~5364&NGC~5317\\
NGC~3611&NGC~3604&          NGC~5371&NGC~5390\\
NGC~3626&NGC~3632&          NGC~5375&NGC~5396\\
NGC~3730&NGC~3732&          NGC~5964&IC~4551\\
NGC~4045&NGC~4046&          NGC~6014&IC~4586\\
NGC~4178&IC~3042&           NGC~6902&IC~4948\\
NGC~4189&IC~3050&           NGC~6923&IC~5004\\
NGC~4193&IC~3051&           NGC~6925&IC~5015\\
NGC~4212&NGC~4208&          NGC~7140&NGC~7141\\
NGC~4310&NGC~4338&          NGC~7552&IC~5294\\
NGC~4319&NGC~4345&                  &\\
\hline
 \end{tabular}
 \tablefoot{The sources used for compiling this table are The Historically Corrected New General Catalogue (HCNGC), NED, and HyperLeda. All double identifications are confirmed by two of those sources except that for NGC~3730 and NGC~3732 (only reported in HyperLeda) and NGC~2974 and NGC~2652 (only reported in the HCNGC).}
\end{table}
